# Supplementary material for: A Vision Check-up for Language Models
Source: arXiv:2401.01862 source file (2024-01-03)
Supplement: Supplementary file 1 [file 10_appendix.tex]

The supplementary file describes in detail the experiments from the main paper, as well as provides additional analysis results. Please refer to the \href{http://vision-checkup.csail.mit.edu}{project webpage} for many additional visual results.

\tableofcontents
\newpage

\section{Experimental settings}
This section provides additional experimental details about the generation and the recognition tasks described in the main paper, including a brief note on the computational resources.

\subsection{Generation}

\paragraph{Prompting Details.}
In all our generation experiments, we supplement the instruction to the model with the following information: ``\emph{You are a helpful assistant and an excellent programmer. You output a code in the programming language} \texttt{[Language Program]} \emph{that draws what the user asks to draw}''. For GPT-4 and GPT-3.5 we inserted this additional instruction through the system prompt. For Davinci this was added at the beginning of the prompt. For all models, we then use the prompt ``\emph{write a code that draws} \texttt{[concept]}''.

\paragraph{2AFC.} 
In our 2AFC experiments, we compare images that render 300 different concepts-- 100 concepts from each category (shapes/objects/scenes), across all models and programming languages (a total of more than 20k images). Before starting the test, workers were presented with a practice session including two trials in the same structure as the test trials, but with no record taken. During the test session, to ensure high-quality responses, each worker was presented with 10 sentinel trials (in addition to the 50 test trials). The sentinel trails include images that depict a simple concept (\eg ``a blue circle''), each paired with an image that does not render that concept. We filter out workers with less than 80\% sentinel accuracy. The 2AFC interface is presented in Fig~\ref{fig:2afc_interface}.

\paragraph{IRB Disclosure.}
We received IRB approvals for our AMT experiments from all of the institutions involved. Accordingly, we took measures to ensure participant anonymity and refrained from showing them potentially offensive content.

\begin{figure}[h]
    \centering
    \includegraphics[trim=0 100 0 100,clip,width=0.7\linewidth]{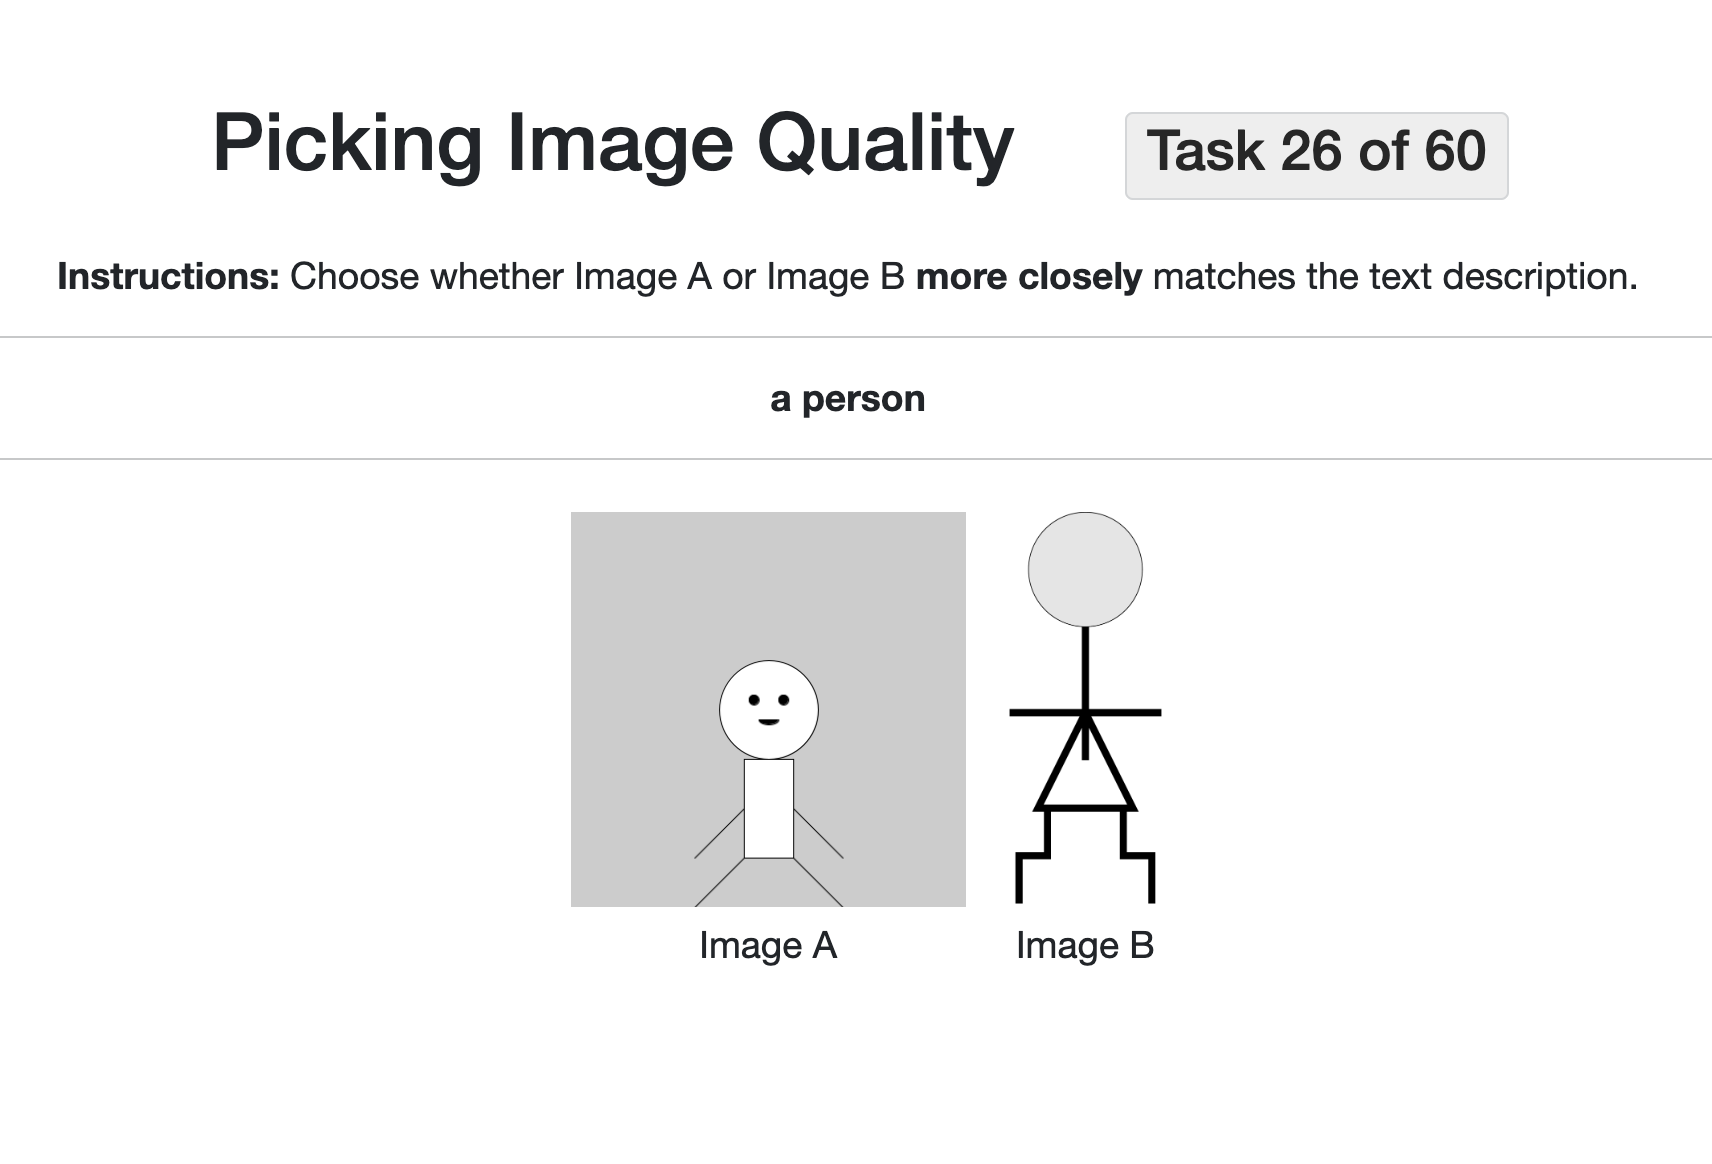}
    \caption{\textbf{2AFC interface.}}
    \label{fig:2afc_interface}
\end{figure}

\paragraph{Image-text retrieval with CLIP score.}
We calculate the agreement of the generated images and the caption of its prompt using CLIP score.
As shown in Fig.~\ref{fig:retrieval}, we first calculate the CLIP scores of the generated images with the possible captions of the visual concepts within the same category (shapes/objects/scenes) and report the rank of the ground-truth caption in percentage (\eg a score of $100\%$ implies that the ground-truth concept is ranked first). 
We found that empirically, CLIP-scores are much more accurate in scoring the draw content if the textual description of the concept is preceded by ``\emph{a clipart of} \texttt{[concept]}''. 

\newpage
\paragraph{CLIP's ability to process LLM’s images.}
We rely on CLIP to assess the fidelity of the generated images with the prompt. The generated images are out-of-distribution compared to the natural images that CLIP was trained with. 
To test whether CLIP is a good indicator in our case, we bring here the agreement between clip rankings and human preference from our 2AFC studies. To do this, we repeat the 2AFC test but replace the human voter with clip rank as a voter (i.e. we compare the clip rank of the two presented images and take clip vote for the higher). Clip rank and human preference are highly correlated with the Spearman correlation score of 0.816 (with p-value=1.25e-09). That means CLIP ranking is a good indicator for image fidelity in our case as well, and that the CLIP ranks reflect user preference. 
Note that this correlation is also important and validates CLIP as a direct indicator, whereas the 2AFC is a comparative test. Ideally, human preferences will be collected as a direct ranking and not with 2AFC, however, such a setting is very noisy as it contains non-calibrator subjective bias, and therefore is usually avoided. 

\begin{figure}[h]
    \centering
    \includegraphics[width=0.4\linewidth]{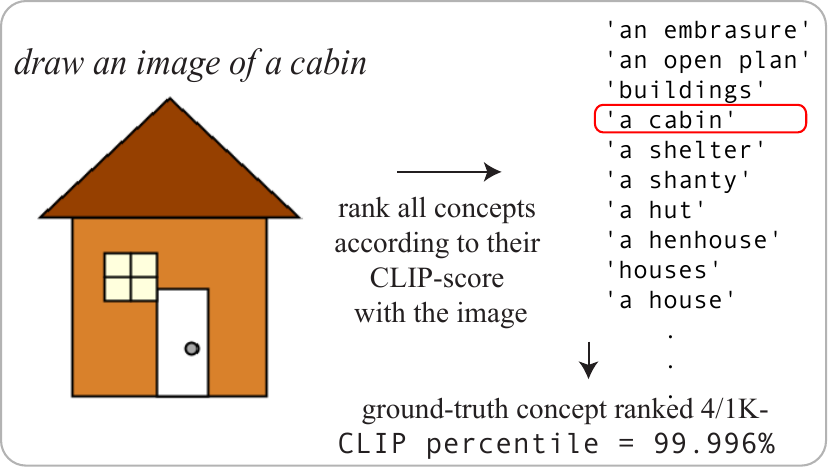}
    \caption{\textbf{Image-text retrieval with clip-score.}}\label{fig:retrieval}
\end{figure}

\paragraph{Using ranking for evaluation.}
Our corpse of captions is highly diverse, but at the same time large enough to contain semantically similar captions. To demonstrate this, we bring here examples of randomly picked concepts and their nearest neighbors in our corpse (based on CLIP text embeddings) in Tab.~\ref{tab:NN_object} and \ref{tab:NN_scenes}. As can be seen, all these concepts have semantically close nearest neighbors. We thus conclude that this dataset is challenging enough to serve as our ranking corpse.

\begin{table}[h]
    \centering
    \begin{tabular}{lc}
         Concept	& Nearest neighbors   \\
         \toprule
         person player  & player, person playing, person, person model, person standing, people \\
         Mineral		   & rock, stone, rocks, glass, object, rocky mountain \\
        Plant pot	    & potted plant, plant pots, planter, plant, pot, bucket, plants \\
        Van side	    & van, car side, bus side, truck, bus, car front \\
        Cans		    & can, tin, canister, boxes, packs, paper cups \\
        Text			& paper, picture, post, cue, book, mobile \\
        Washing-machines& dishwasher, washbasin, clothes, machinery, oven, sewing machine \\
        Bicycle			& motorbike, car, cart, aircraft, truck, wheel \\
        Dresser			& drawer, drawers, chest of drawers, sideboard, cabinet, cupboard \\
        tracks			& track, railway, train, dirt track, cars \\
        \bottomrule  
    \end{tabular}
    \caption{\textbf{Nearest neighbor evaluation for object dataset}}
    \label{tab:NN_object}
\end{table}

\begin{table}[h]
    \centering
    \begin{tabular}{p{0.45\textwidth}|p{0.55\textwidth}}
    Concept & Nearest neighbors \\
    \toprule
    A table full of vegetables and fruits piled on top of each other. & A small wooden table covered with delicious vegetables. \newline a bowl of fruit and pastry on a table \newline 
    mixture of fruits kept in a big bowl \newline a counter with vegetables, knife and cutting board on it. \newline Fruit and vegetables are hanging in a metal basket. \\
    \hline
    A kitchen with a washer sitting next to a metal sink. & A view of a kitchen with cabinets, a sink and a clothes washer. \newline An oven in a kitchen with a stove on top in between counter tops. \newline A kitchen with a wooden counter next to an oven with a stove. \newline a kitchen with a refrigerator a sink and a stove \newline a kitchen with a sink a stove and a microwave \\
    \hline
    An intracately designed boat on a river bank. & A boat that looks like a car moves through the water. \newline A large boat filled with mean on wheels. \newline The sightseeing boat streams along the river joined by a plane \newline A house boat along the water has bicycles on deck. \newline An airplane with its landing wheels out landing. \\
    \hline
    A man standing next to a set of piked motorcycles. & Man in motorcycle leathers standing in front of a group of bikes \newline A middle aged man standing next to a parked motorcycle \newline A young boy stands next to a row of parked motorcycles. \newline A man standing next to a motorcycle in the middle of a street. \newline A man stands next to a motorbike on some pavement. \\
    \hline
    A walk in shower next to a toilet with a wooden seat. & A bathroom with a walk in shower next to a toilet. \newline An empty bathroom with a shower next to a toilet. \newline A bathroom with a sliding shower door next to a toilet. \newline A bathroom with an enclosed shower door next to a toilet. \newline A bathroom with an enclosed shower next to a sink and a toilet. \\
    \hline
    A crowd of bikers driving down a street next to tall buildings. & A large number of people riding motorcycles down the road. \newline A motorcycle rally on the street with many spectators. \newline A group of motorcyclists driving down the road. \newline A group of bikers riding down the road together. \newline two lines of motorcycles driving down the road while a crowd watches \\
    \bottomrule
    \end{tabular}
    \caption{\textbf{Nearest neighbor evaluation for scene dataset}}
    \label{tab:NN_scenes}
\end{table}

\newpage
\subsection{Recognition}

\paragraph{Human drawing.}
In order to assess the ability of LLMs to recognize human drawings, we built a dedicated interface that allows users to select simple shapes and colors to draw a desired concept. When the drawing process is done, the tool allows transferring each of the human drawings into a processing code that renders it. A print-screen of the tool is available in Fig.~\ref{fig:drawing_interface}.
We launched our interface on Amazon Mechanical Turk. We randomly sample 100 concepts from each category used in our recognition experiments (objects/scenes). Each worker was first presented with a practice trail, allowed to explore the drawing tool, and was then asked to draw 20 concepts with a limited time of 2 minutes for each. In total, we collected 1200 drawings (600 from each category). To ensure only high-quality results, we include sentinel tests where we ask the users to draw a simple concept (\eg a blue circle). Each user was presented with 3 sentinels tests, and we filtered out users that drew more than 2 sentinels incorrectly. As in all our recognition experiments, we also filtered out drawings with an image-text retrieval score of less than 96\%. After filtering, we were left with 162 and 113 object and scene drawings respectively. Examples of human drawings are available in Fig.~\ref{fig:human_drawings}. 

\begin{figure}[h]
    \centering
    \fbox{\includegraphics[width=0.4\linewidth]{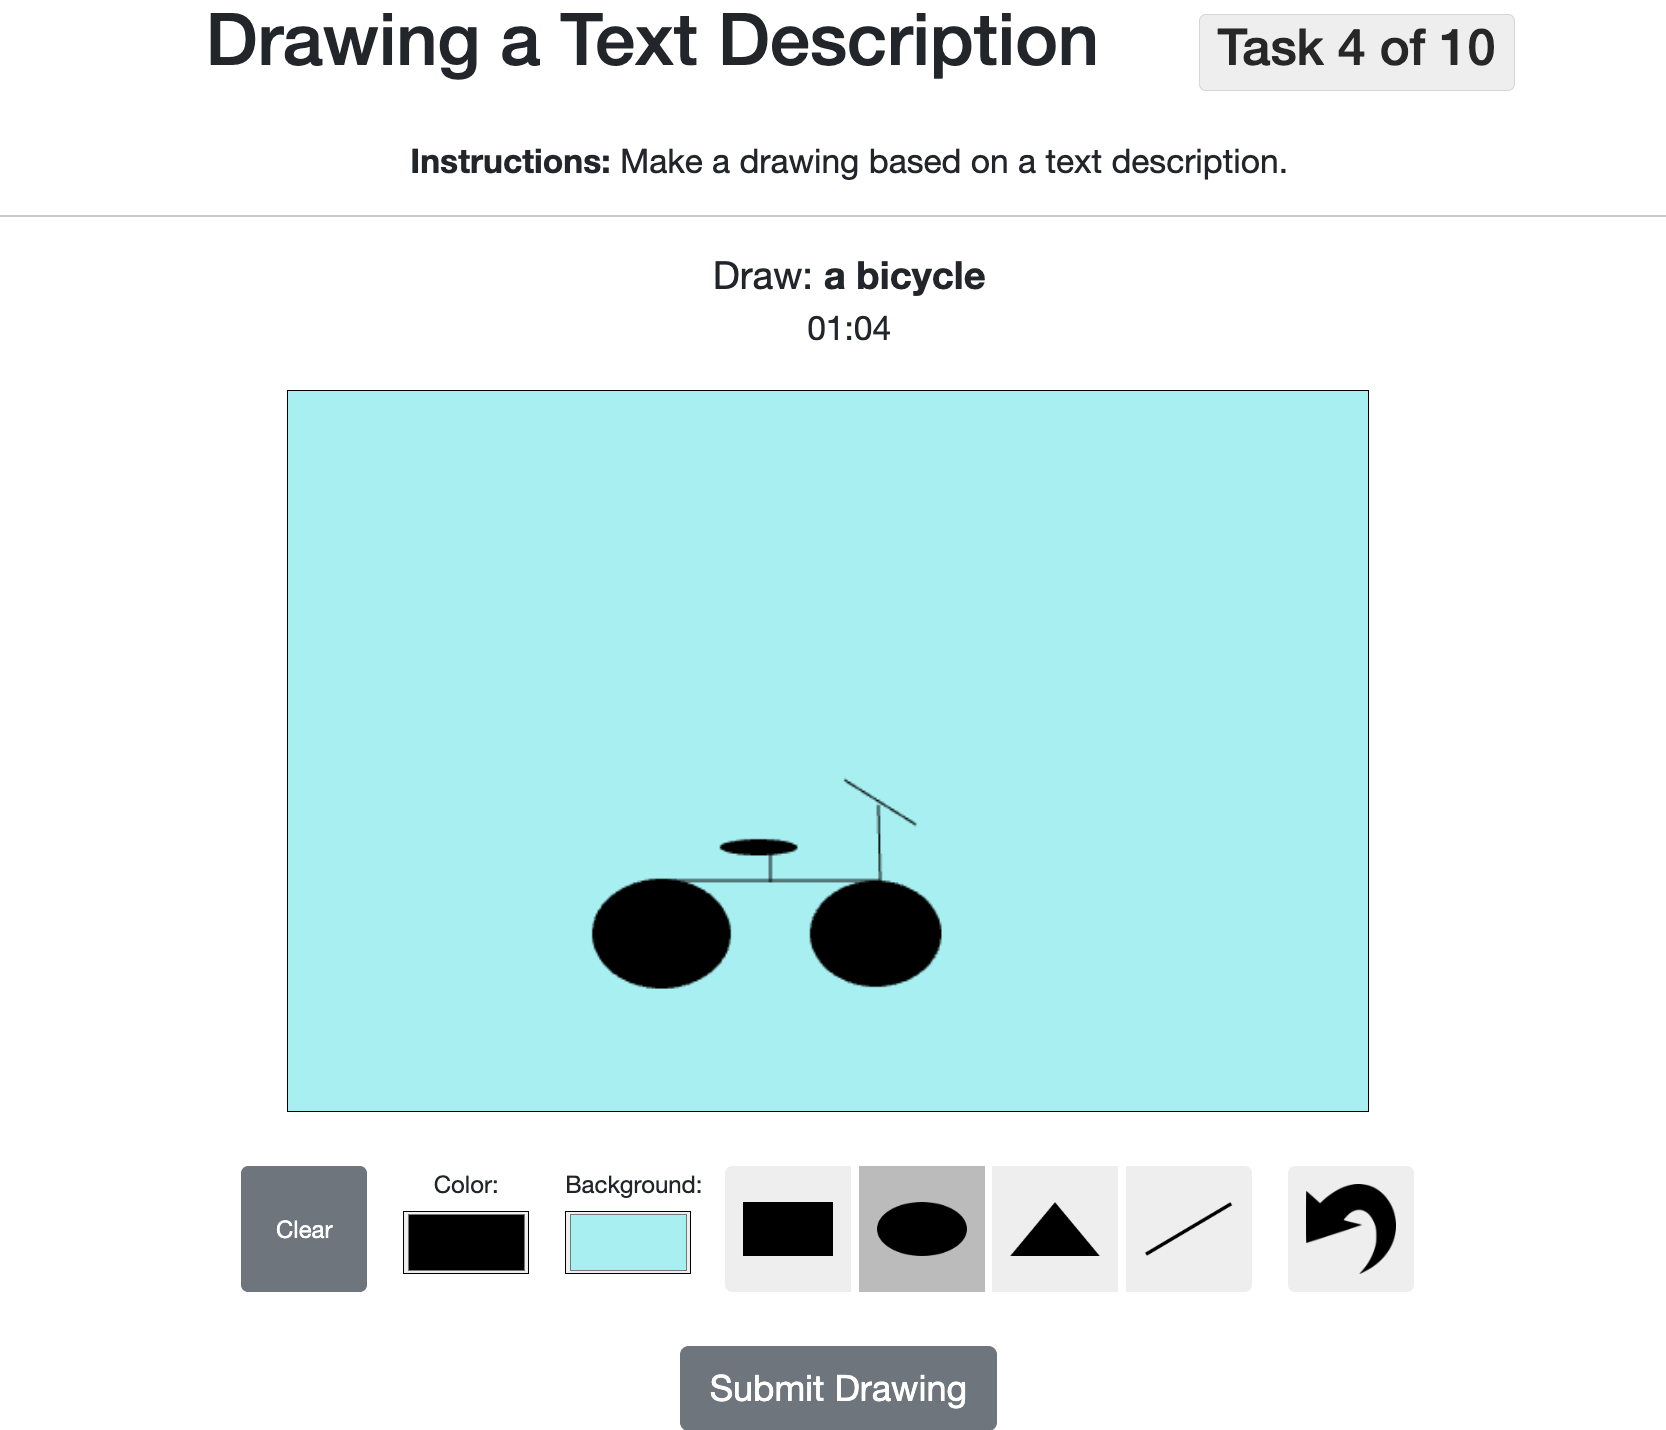}}
    \caption{\textbf{Drawing Interface.} Our interface allows users to draw the desired concept with simple shapes and colors.}
    \label{fig:drawing_interface}
\end{figure}

\begin{figure}[h]
    \centering
    \includegraphics[width=0.98\linewidth]{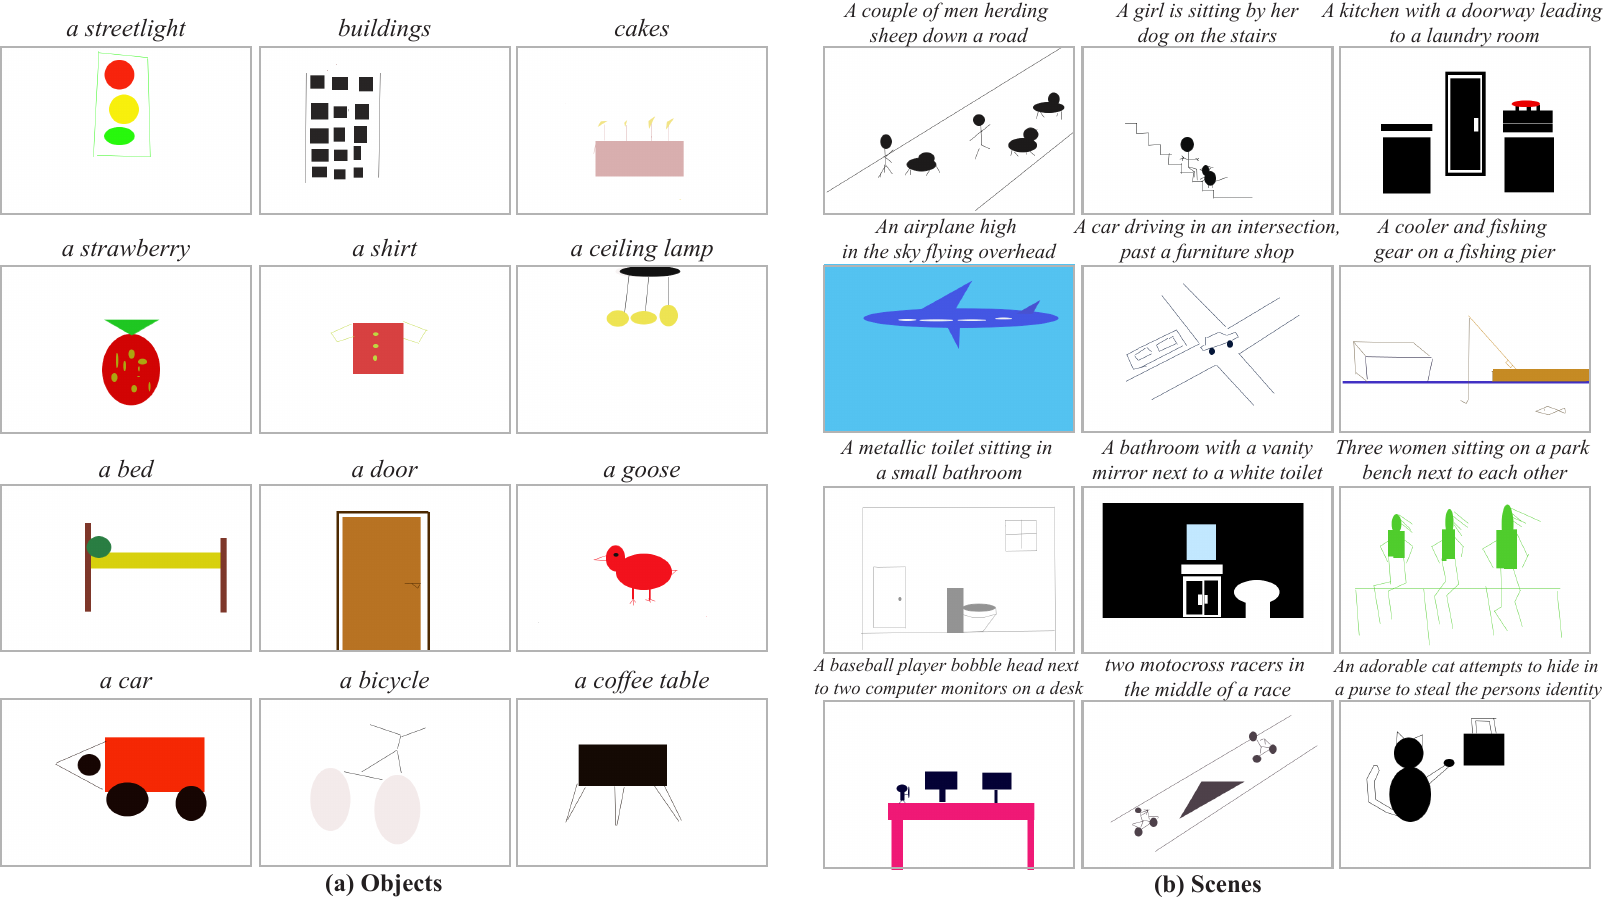}
    \caption{\textbf{Human drawings:} Examples of drawings collected from users by our drawing interface that passed the sentinel and CLIP score filtering. Each of the collected drawings is transferred into a processing code, and then included in the LLMs' recognition tests.}
    \label{fig:human_drawings}
\end{figure}

\subsection{Computation Resources.} 
Our experiments were conducted by using the python API provided by Open-AI. We use this to interact and collect responses from the tested LLMs. This enables us to test different models and different programming languages, and to run multiple experiments in parallel.

\newpage
\section{Additional Analysis}
In this section, we provide some additional analysis and results, including a random subset of visual results.  

\newpage
\subsection{Generation}

\paragraph{Failure cases.}
Although in general, all models are successful in accurately generating visual concepts according to textual instructions, in some cases even relatively simple concepts are difficult for the models to draw. We identify several failure modes, as seen in Fig~\ref{fig:gen_fail}: (a) the drawing is very sparse and low in detail, (b) the representation is partial-- the drawing is either corrupted (\eg the T-shirt drawing), or represents only some of the concepts (a typical failure reason for the scenes dataset) and (c) the model is unable to draw certain categories, like digits. With all models and languages, we found the task of drawing digits to be surprisingly challenging.  

\begin{figure}[h]
    \centering
    \includegraphics[width=1\textwidth]{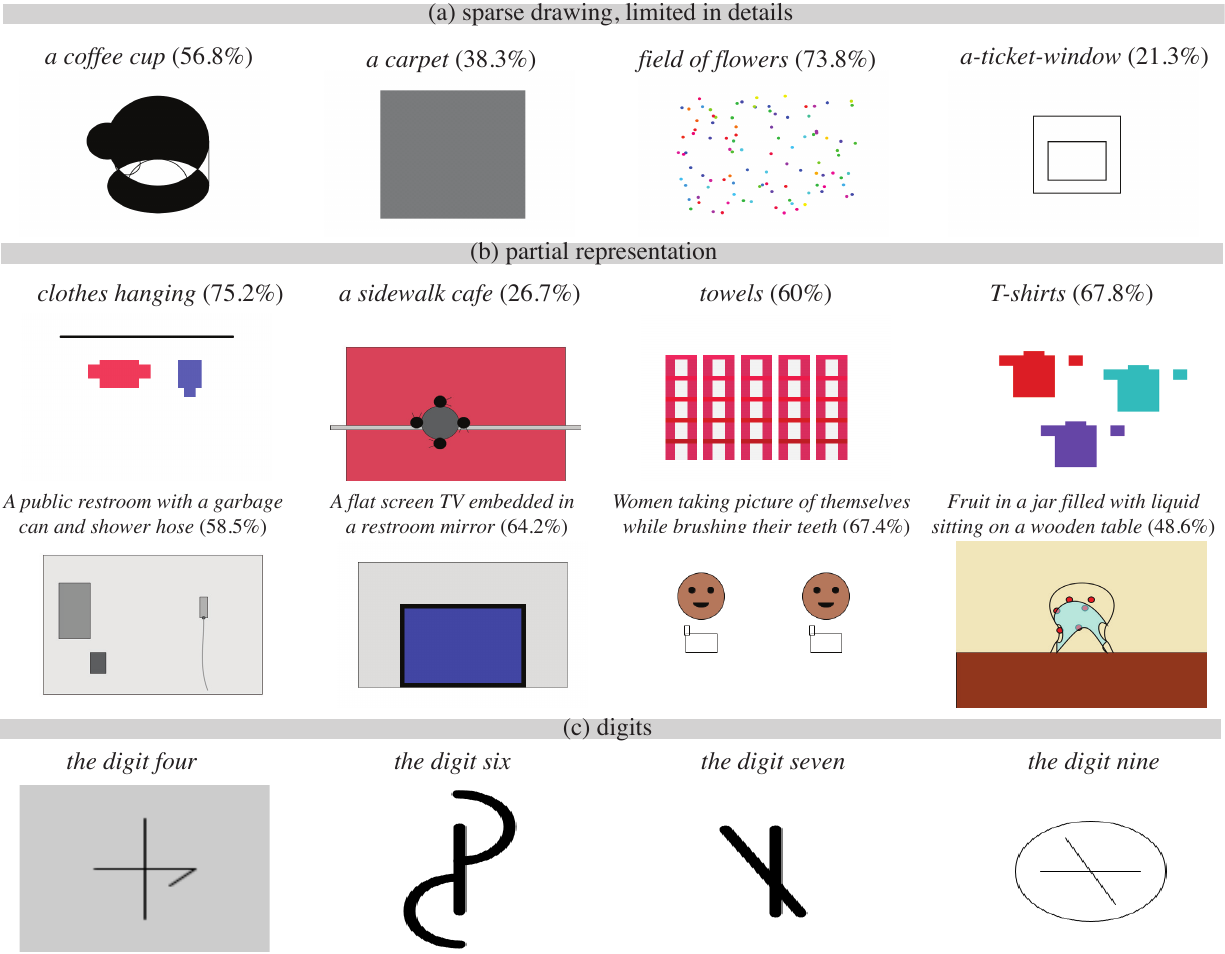}
    \caption{\textbf{Generation failure cases.} Scores in brackets report the CLIP image-text retrieval rank (higher is better).}
    \label{fig:gen_fail}
\end{figure}

\newpage

\paragraph{Effect of prompting.}
We test the effect of prompting with positive reinforcement on the %
rendering competence. We use three levels of reinforcement. No reinforcement, light reinforcement: \texttt{"you are a helpful assistant and excellent programmer"}, and a strong one: \texttt{"The images you've created using code are a testament to your creativity, innovation, and technical expertise"}. 
Positive reinforcement significantly improves the performances of Davinci (Fig.~\ref{fig:possitive}) but is less effective for the other models. Similar behavior can be achieved when executing the task in two stages: models are first asked to describe how to draw the concept, and only then write a code that renders it. An additional interesting prompting effect is by language, which in some cases is
highly entangled with the visual appearance of the results (Fig.~\ref{fig:language}).

\begin{figure}[h]
\centering
\includegraphics[width=0.4\linewidth]{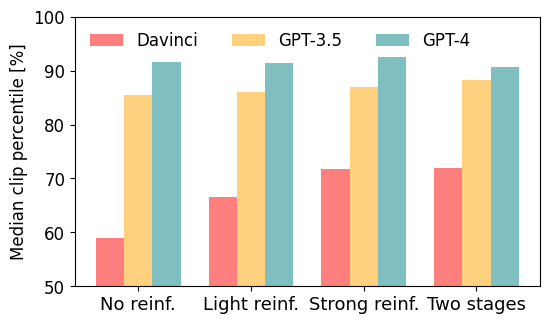}
    \caption{\textbf{The effect of positive reinforcement.}}
    \label{fig:possitive}
\end{figure}

\begin{figure}[h]
    \centering
    \captionsetup[subfigure]{labelformat=empty,justification=centering,aboveskip=1pt,belowskip=1pt}
    \begin{subfigure}[t]{0.24\textwidth}
        \centering
        \caption{English}        \includegraphics[width=0.98\linewidth,height=1.8cm]{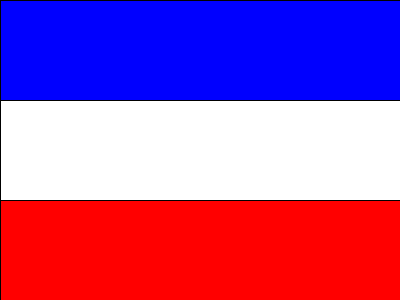}
    \end{subfigure}
    \begin{subfigure}[t]{0.24\textwidth}
        \centering
        \caption{Spanish}        
        \includegraphics[width=0.99\linewidth,height=2.8cm]{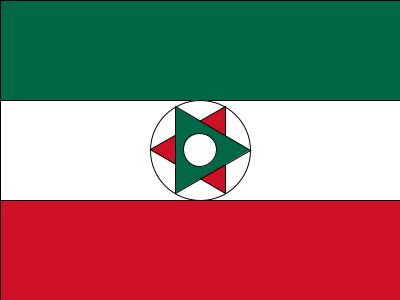}
    \end{subfigure}
    \begin{subfigure}[t]{0.24\textwidth}
        \centering
        \caption{Hindi}
        \includegraphics[width=0.99\linewidth,height=2.8cm]{figures/cultural-bias/झंडा_0.png}
    \end{subfigure}
    \begin{subfigure}[t]{0.24\textwidth}
        \centering
        \caption{Chinese}
        \includegraphics[width=0.99\linewidth,height=2.8cm]{figures/cultural-bias/旗帜_0.png}
    \end{subfigure}
    \par\smallskip
        \begin{subfigure}[t]{0.24\textwidth}
        \centering
        \includegraphics[width=0.98\linewidth,height=2.8cm]{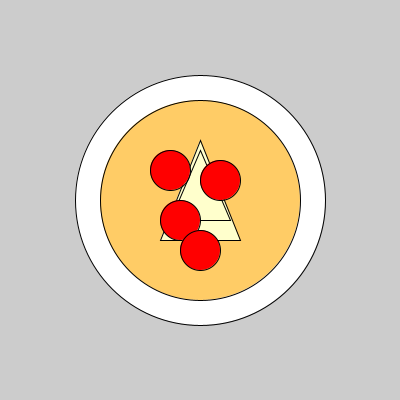}
    \end{subfigure}
    \begin{subfigure}[t]{0.24\textwidth}
        \centering
        \includegraphics[width=0.99\linewidth,height=2.8cm]{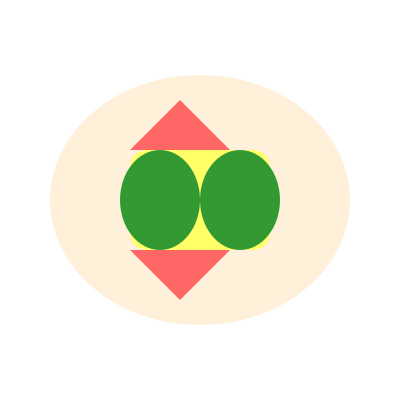}
    \end{subfigure}
    \begin{subfigure}[t]{0.24\textwidth}
        \centering
        \includegraphics[width=0.99\linewidth,height=2.8cm]{figures/cultural-bias/खाना_0.png}
    \end{subfigure}
    \begin{subfigure}[t]{0.24\textwidth}
        \centering
        \includegraphics[trim= 50 120 50 0,clip,width=0.99\linewidth,height=2.8cm]{figures/cultural-bias/一顿饭_0.png}
    \end{subfigure}
    \caption{\textbf{The effect of language.} We ask the GPT-3.5 to draw a flag and a meal in four different languages. Surprisingly, the language used has a compelling effect on the generated content, hinting for cultural bias. This may hint that the model hold some visual cultural bias. %
}
    \label{fig:language}
\end{figure}

\newpage

\paragraph{Image-text fidelity.}
Below is the full image-text fidelity analysis for all programming languages, models, and categories. More complicated concepts, like complex scenes, are more difficult to draw; therefore, their fidelity scores tend to be lower. Not surprisingly, GPT-4 outperforms GPT-3.5 and Davinci. Overall, processing is the preferred programming language by all models.  

\begin{figure}[h]
    \centering
    \includegraphics[width=1\linewidth]{figures/clip_bar.pdf}
    \caption{\textbf{Image-Text Fidelity.} Median CLIP image-text retrieval percentiles of images generated by different \acp{LLM}. We include Stable Diffusion as an Oracle. Chance is $50\%$.}\label{fig:clip-all}
    \vspace{-1.2em}
\end{figure}

\paragraph{Human perceptual study.}
We report here the full results of the ``two alternative force choice'' studies presented in the main text. Figure~\ref{fig:2afc} presents the mean preference rate that each model and programming language achieves on each of the three concept categories (shapes/objects/scenes). On average, for all categories, GPT-4 is preferred over GPT-3.5 which is preferred over Davinci, with tikz and processing preferred over turtle and matplotlib. Error bars indicate the variance calculated by the bootstrap algorithm with 10k steps.

\begin{figure}[h]
    \centering
    \begin{subfigure}[t]{0.35\textwidth}
    \includegraphics[trim=0 0 40 0,clip,width=0.98\linewidth, height=3.7cm]{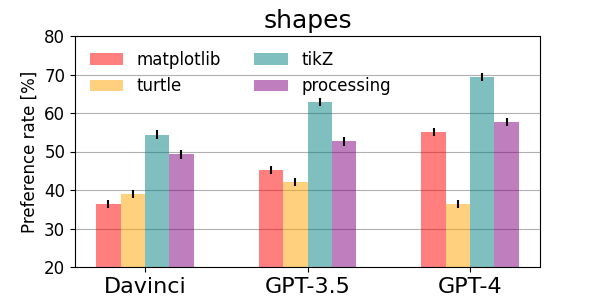}
    \end{subfigure}
    \begin{subfigure}[t]{0.31\textwidth}
    \includegraphics[trim=50 0 40 0,clip,width=0.98\linewidth, height=3.7cm]{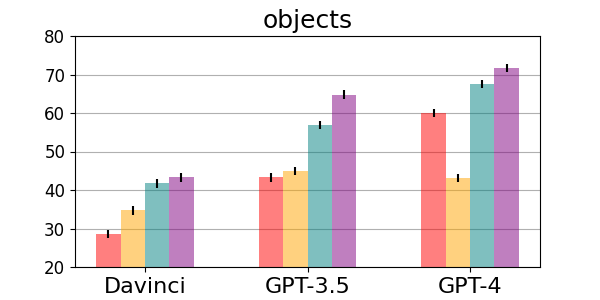}
    \end{subfigure}
    \begin{subfigure}[t]{0.31\textwidth}
    \includegraphics[trim=50 0 40 0,clip,width=0.98\linewidth, height=3.7cm]{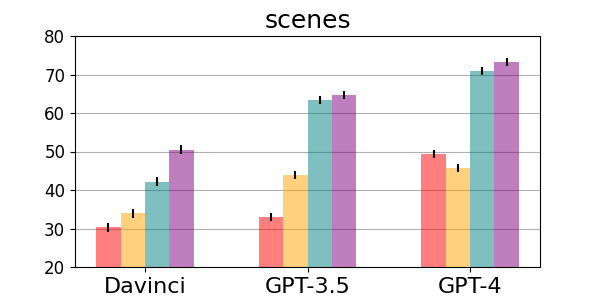}
    \end{subfigure}
    \caption{\textbf{Human perceptual study.} Error bars report the variance estimated by bootstrap.} \label{fig:2afc}
    \label{fig:my_label}
\end{figure}

\newpage

\paragraph{Realism.}
We evaluate the realism of the generated drawings using the FID score, compared with 1K random images from ImageNet. Table~\ref{tab:realism_fid}(a) presents the FID scores (higher is better) for all models, languages, and data categories (shapes/objects/scenes). For all cases, FID scores are relatively high, indicating that the images are far from being natural. Interestingly, GPT-4 scores are on average better than the other models.

\paragraph{Diversity.}
In the main text, we show how LLMs can generate various drawings of the same concept, indicating they hold a visual representation of the concept. 
In Table~\ref{tab:realism_fid}(b) we report the LPIPS diversity scores of all models and programming languages, averaged on 5 samples for each of the 100 concepts randomly chosen from the ``objects'' category. We tested two drawing approaches: (i) sampling new drawings by sequential prompting the model to draw the same concept (drawing sample), and (ii) prompting the model to write a function that on each call produces a different drawing of the concept (function samples). Results show that both GPT-3.5 and GPT-4 produce more diverse samples than Davinci, and that the strategy (i), sampling directly from the model produces more diverse samples on average than generating a single program from which we can sample at random. 
Note that with tikZ it is impossible to write a function that generates different drawings, as the syntax does not support random variables .

\begin{table}[h]
    \centering
    \resizebox{1\columnwidth}{!}{%
    \begin{tabular}{cc}
    \begin{tabular}{lcccccc}
        \toprule
        task & model & matplotlib & turtle & tikZ & Processing
        \\
        \midrule
        \multirow{3}{30pt}{shapes} 
        & Davinci & 217.8 & 194.8 & 238.6 & 230
        \\
        & GPT-3.5 & 195.8 & 195.4 & 206.2 & 210.5
        \\
        & GPT-4 & \textbf{186.2} & 193.7 & 205 & 193.5 
        \\
        \midrule
        \multirow{3}{30pt}{objects} 
        & Davinci & 251.1 & 208.4 & 259.8 & 244.5
        \\
        & GPT-3.5 & 240.4 & 187.6 & 197.4 & 177.9 
        \\
        & GPT-4 & 194.8 & 185.6 & 211.3 & \textbf{172.7}
        \\
        \midrule
        \multirow{3}{30pt}{scenes} 
        & Davinci & 271.6 & 230.9 & 237.6 & 229
        \\
        & GPT-3.5 & 241.3 & 204.6 & 201.6 & 201.3
        \\
        & GPT-4   & 210.9 & 203.7 & \textbf{182.5} & 186.7
        \\
        \bottomrule
    \end{tabular}
&
    \begin{tabular}{lcccccc}
        \toprule
        task & model & matplotlib & turtle & tikZ & Processing
        \\
        \midrule
        \multirow{3}{50pt}{drawing sample} 
        & Davinci & 0.061 & 0.039 & 0.023 & 0.037
        \\
        & GPT-3.5 & 0.464 & 0.244 & 0.261 & 0.482
        \\
        & GPT-4 & 0.302 & 0.182 & 0.233 & 0.404
        \\
        \midrule
        \multirow{3}{50pt}{function samples} 
        & Davinci & 0.188 & 0.104 & - & 0.319
        \\
        & GPT-3.5 & 0.22  & 0.205 & - & 0.263   
        \\
        & GPT-4 & 0.216 & 0.148 & - & 0.224
        \\
        \bottomrule
    \end{tabular}
    \\
    \textbf{(a) Realism (FID $\downarrow$)} & \textbf{(b) Diversity (LPIPS diversity  $\uparrow$))}
    \end{tabular}
    }
    \vspace{0.5cm}
    \caption{Realism and Diversity analysis.} \label{tab:realism_fid}
\end{table}

\paragraph{What visual concepts are more ``drawable''?} To better understand what concepts are easier for the model to draw, we break down the shapes dataset into the different shapes and relation categories, and report the median CLIP percentile for each in Fig.~\ref{fig:gen_analysis}. We also report the median scores for each of the scene categories. We bring the full analysis for all models and language programming in Fig.~\ref{fig:sh} and Fig.~\ref{fig:sc}.
\begin{figure}[htp]
    \centering
    \includegraphics[width=0.6\linewidth]{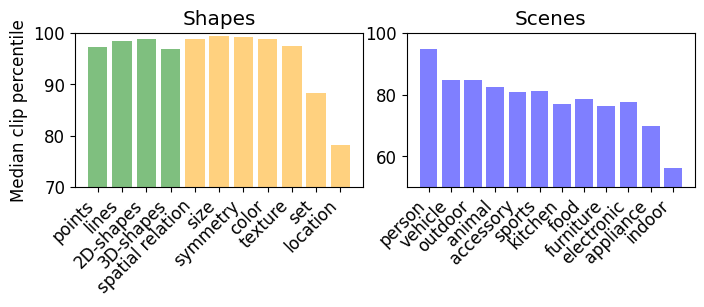}
    \caption{\textbf{What visual concepts are more ``drawable''?}}\label{fig:gen_analysis}
\end{figure}

\newpage
\begin{figure}[h]
    \centering
    \includegraphics[width=\textwidth]{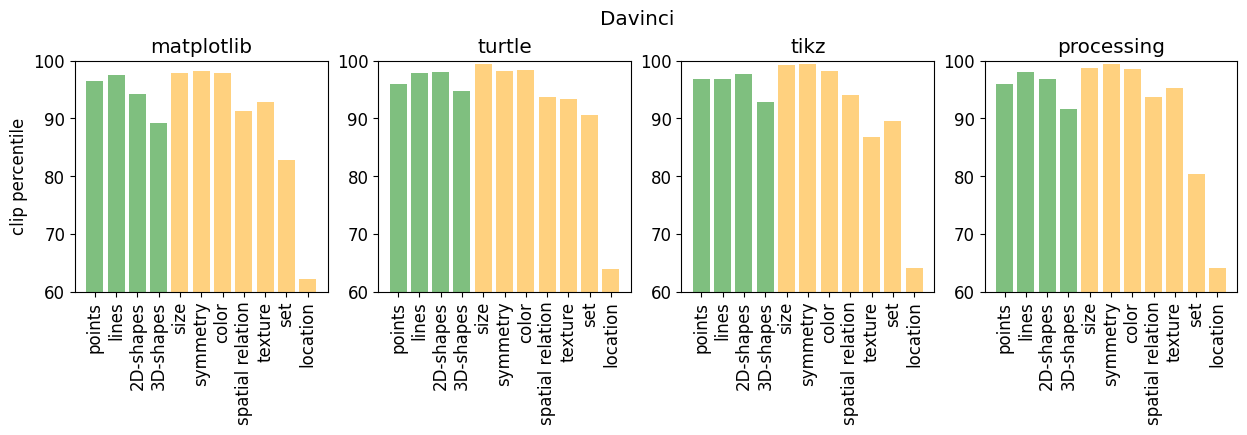}
    \includegraphics[width=\textwidth]{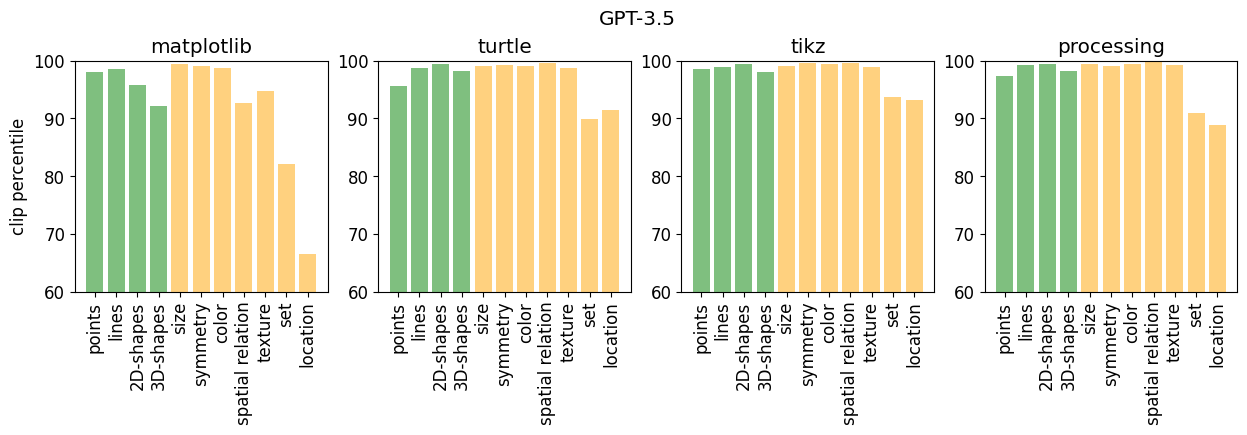}
    \includegraphics[width=\textwidth]{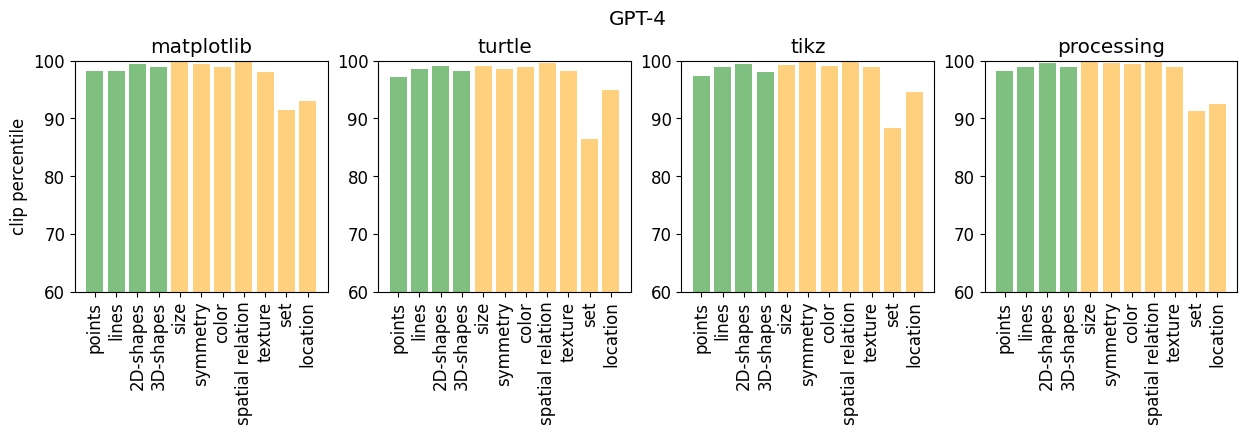}
    \caption{Shape generation, full analysis.}
    \label{fig:sh}
\end{figure}
\newpage

\begin{figure}[h]
    \centering
    \includegraphics[width=\textwidth]{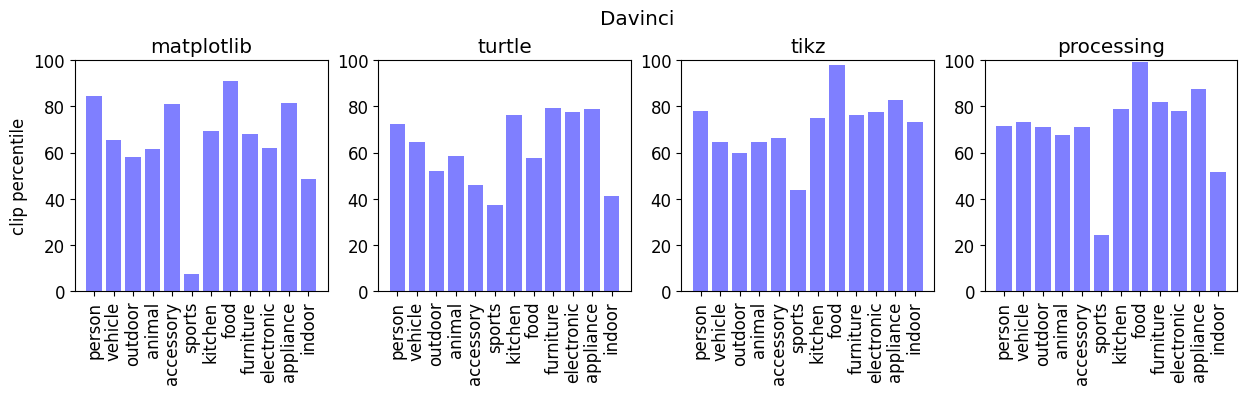}
    \includegraphics[width=\textwidth]{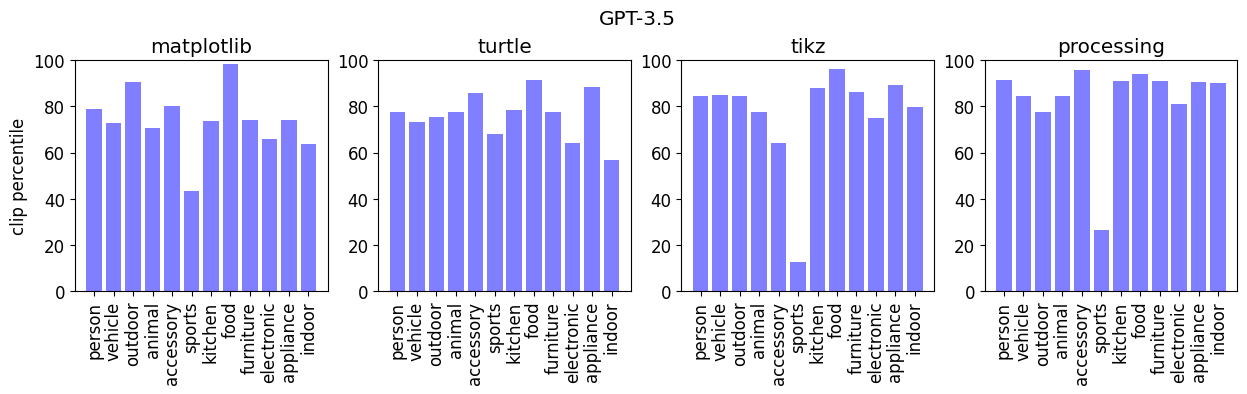}
    \includegraphics[width=\textwidth]{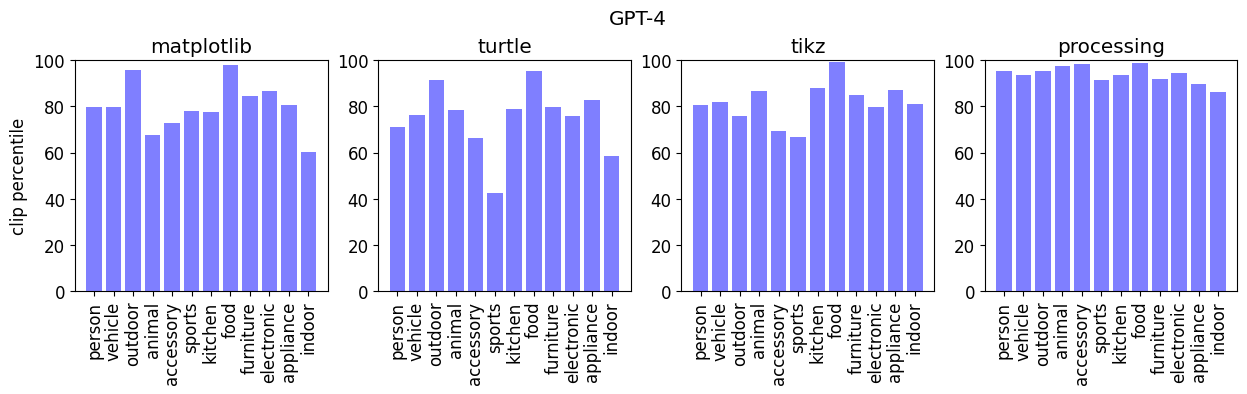}
    \caption{Scene generation, full analysis.}
    \label{fig:sc}
\end{figure}

\newpage
\subsection{Feedback}
In this section, we provide additional analysis of the feedback-augmented text-to-image generation results. 

\paragraph{Feedback improves generation:} Compared to the GPT-4 based visualizations highlighted in the main paper (Fig.~1 and Fig.~7), Fig.~\ref{fig:success-feedback-gpt35} demonstrates feedback-based generation of different shapes using GPT-3.5. As can be seen in Fig.~\ref{fig:success-feedback-gpt35}  Row 2 /  Row 4 / Row 10, the \textit{overall relative placement of shapes} improves with more iterations of the feedback-based generation. Row 6 highlights an example where \textit{the count of the desired shapes} improves with feedback, while Row 3 / Row 10 highlight examples of \textit{structure} improvement over multiple iterations.

\begin{figure}[h]
    \centering    \includegraphics[width=0.58\linewidth]{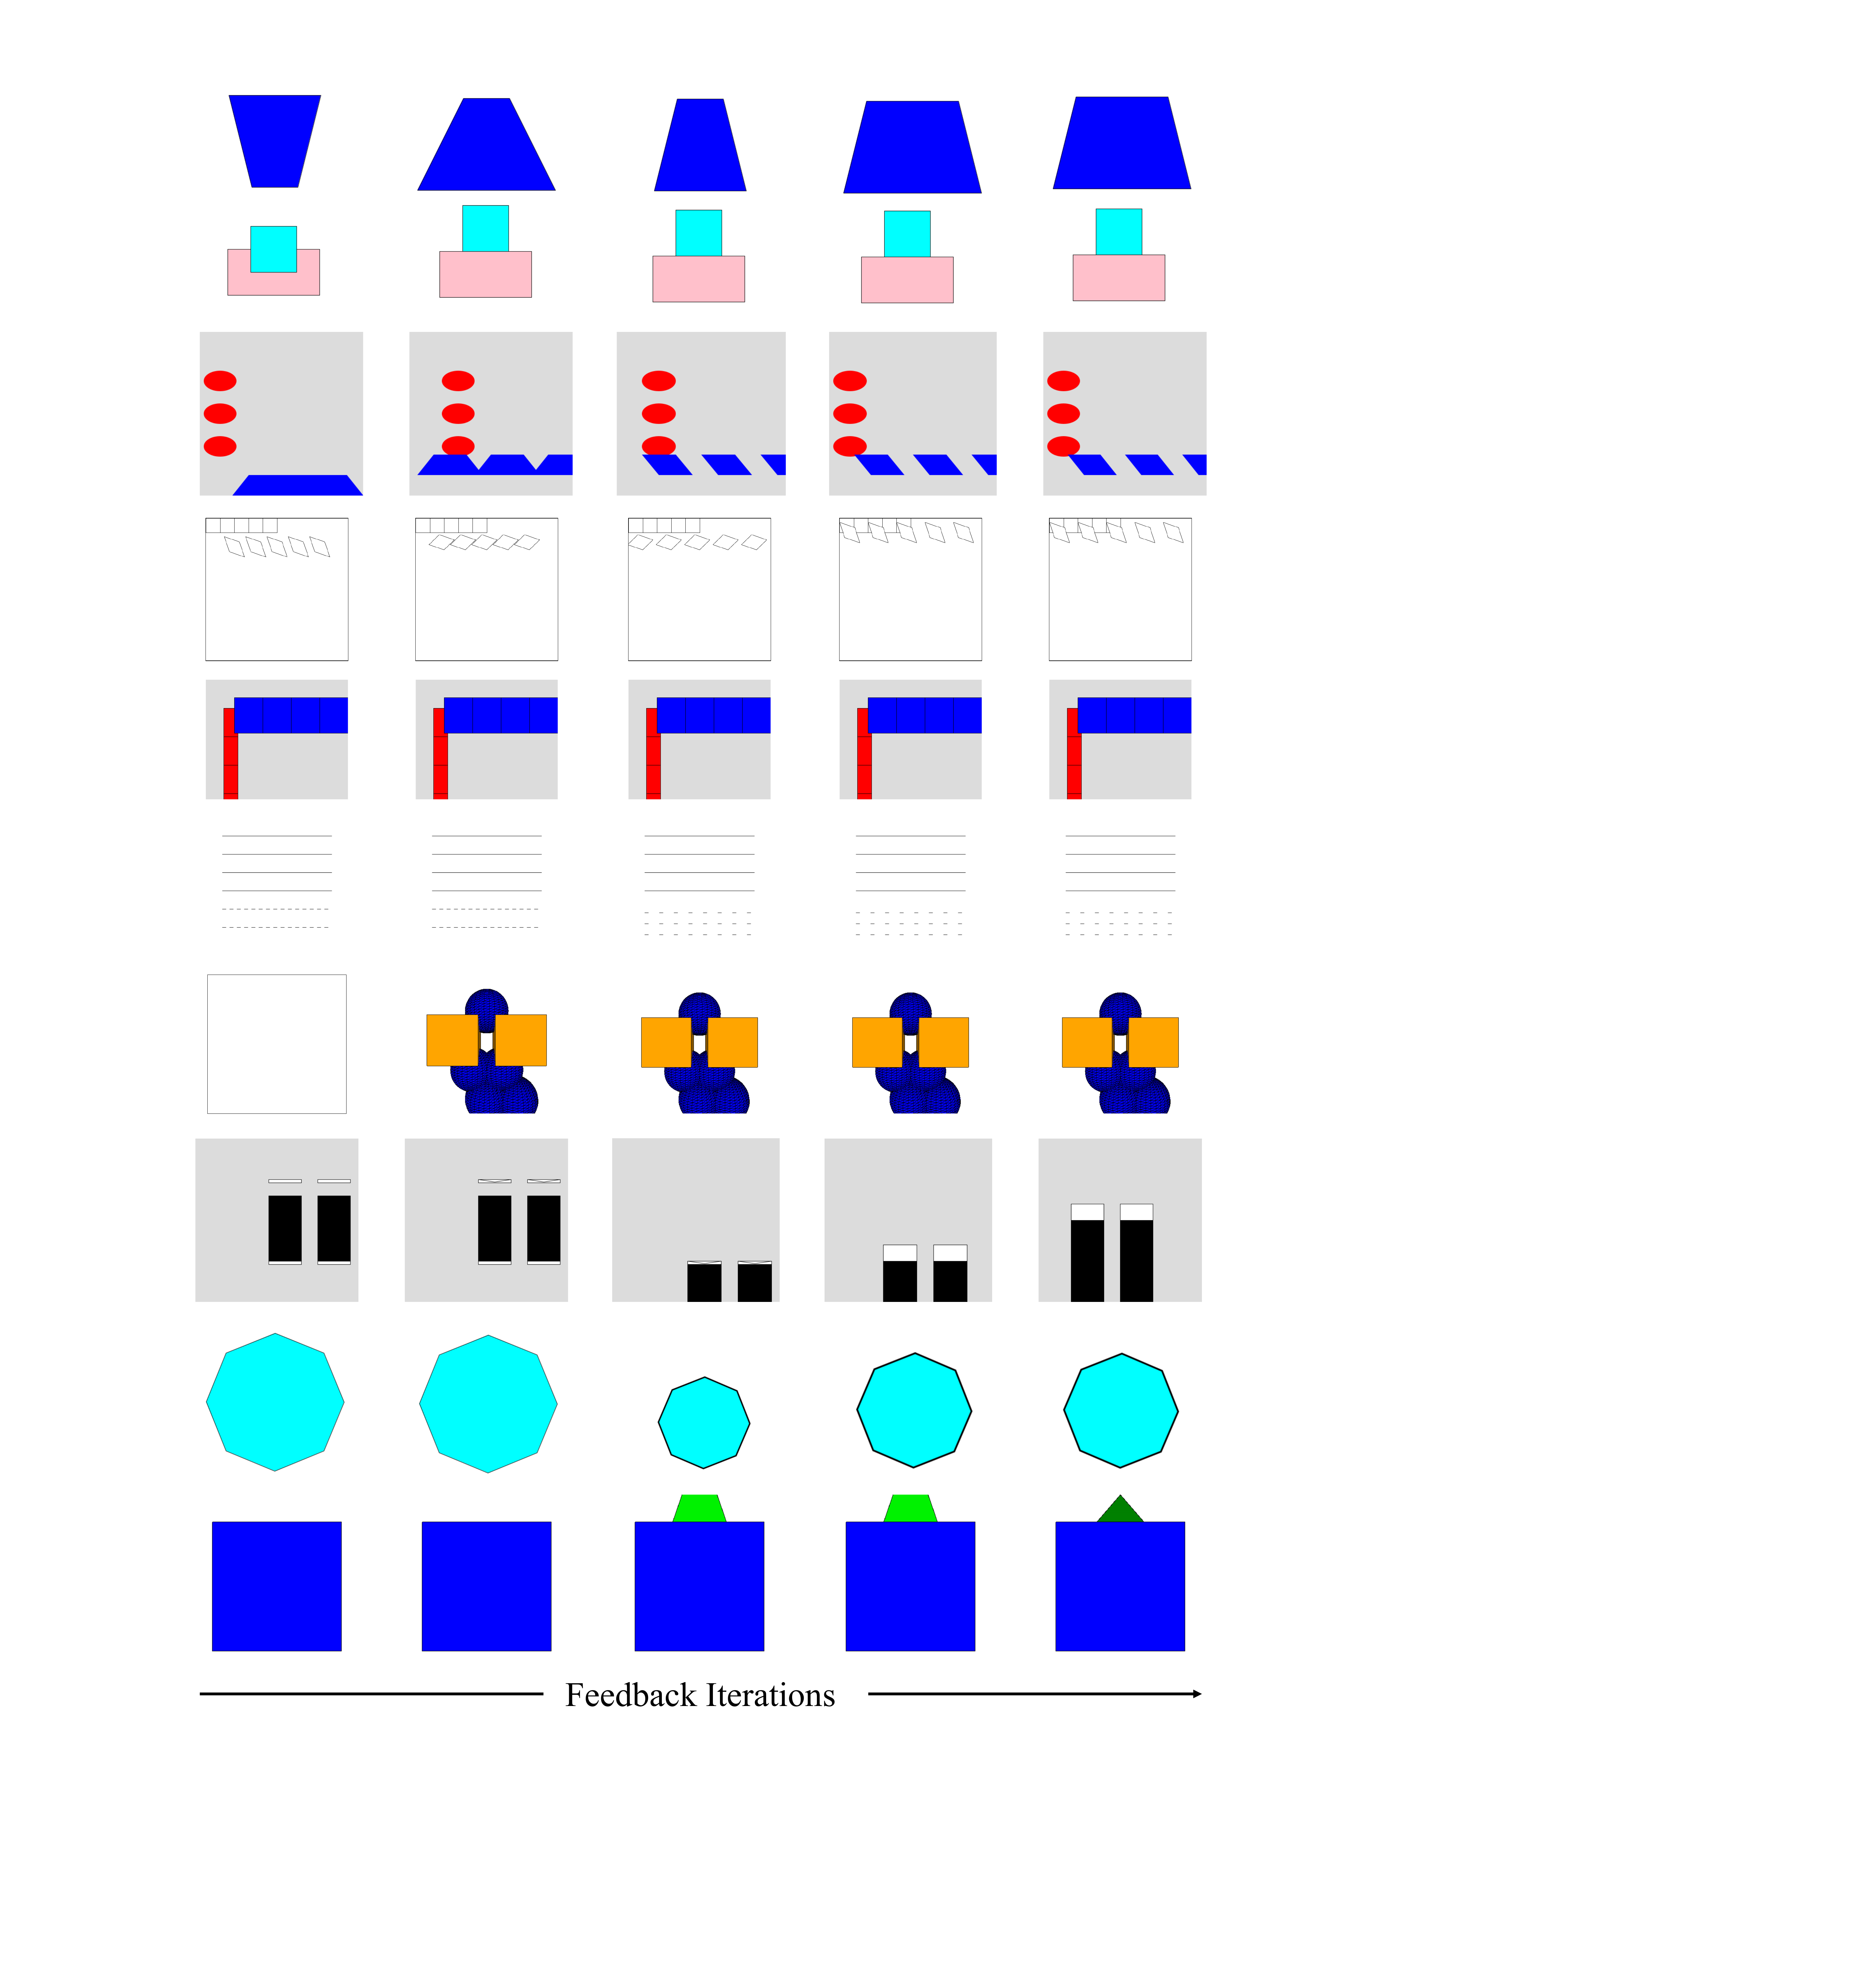}
    \caption{\textbf{Feedback-based Shape Generation using GPT3.5}––– Captions (from top to bottom): \textbf{A} blue trapezium; \textbf{A} cyan square located to the top of a pink rectangle; \textbf{T}hree ovals on the left of the image and three parallelograms on the bottom of the image; \textbf{F}ive rectangles on the top left of the image and five parallelograms on the top of the image; \textbf{F}our tubes on the left of the image and four cubes on the top of the image; \textbf{F}our thin black lines and three dashed black lines; \textbf{T}wo orange prisms and five blue spheres; \textbf{T}wo tubes on the bottom right of the image; \textbf{A} cyan octagon; \textbf{A} green prism on top of a blue cube.}
    \label{fig:success-feedback-gpt35}
\end{figure}

\newpage
\paragraph{Feedback hurts generation –– Failure cases:} 
We analyze the typical failure cases for feedback, exemplified in Fig.~\ref{fig:failures-feedback}: (a) Skipping between modes: the model ``restarts'' the drawing every few iterations. For example in the first line of Fig.~\ref{fig:failures-feedback} the model starts out drawing a bat, initiates a new "mode" of plausible drawing of a bat, corrects it for a few steps, and then restarts again. (b) Non-monotonic improvement: this is exemplified by the bottle drawing in Fig.~\ref{fig:failures-feedback}, where the model starts with drawing a container, but the image worsens before it improves. This phenomenon can be also seen in the case of the bucket, where the model produces a reasonable drawing that is then made worse with additional corrections. (c) The model fails to represent the concept: in this case, the model fails to accurately draw the concept (\eg ``a clothespin''), even with multiple feedback rounds. The last failure mode is also present when drawing digits, for which multiple rounds of feedback cannot properly draw them, as seen in Fig.~\ref{fig:failures-digits}.

\begin{figure}[h]
    \centering    \includegraphics[width=0.7\linewidth]{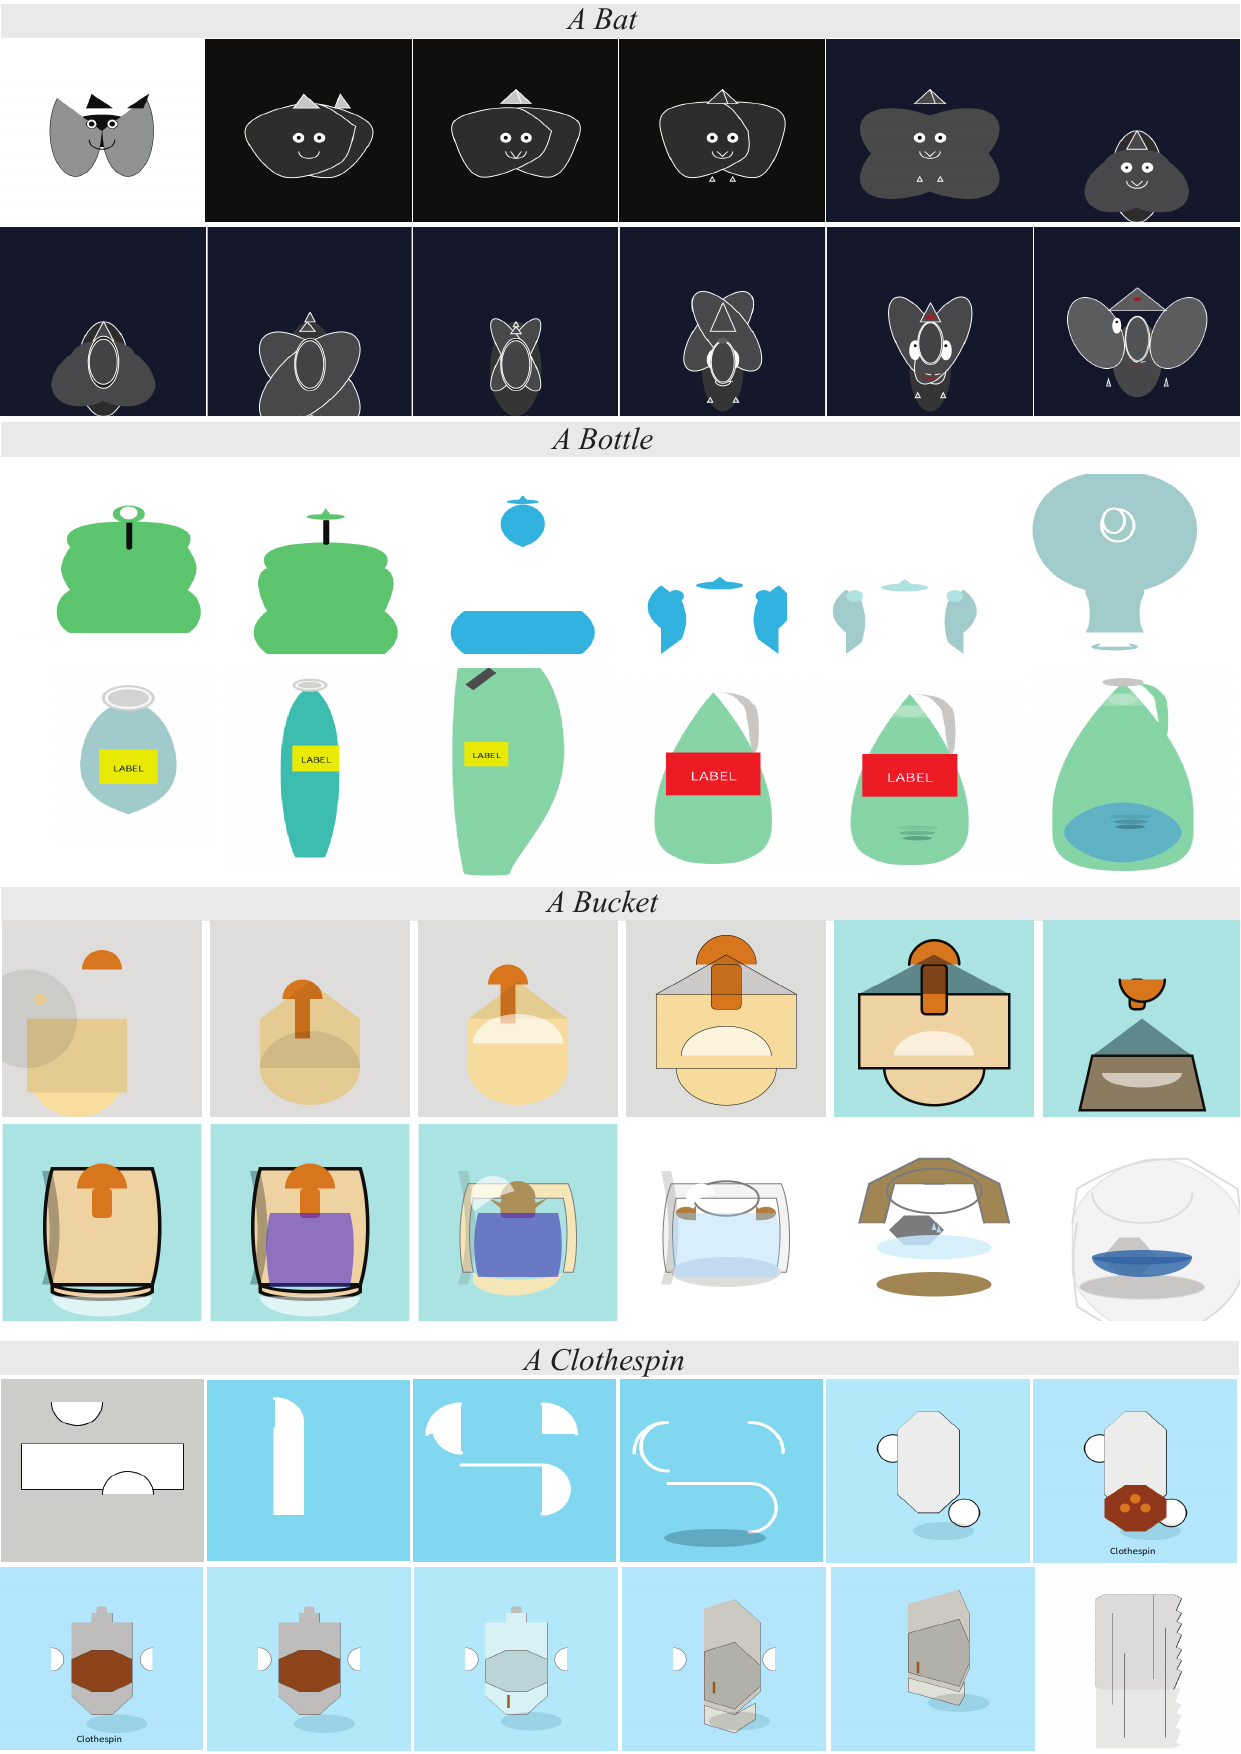}
    \caption{\textbf{GPT 3.5: Feedback failure cases.} Three failure cases when drawing a bat, a bottle and clothespin a clothespin using feedback. }
    \label{fig:failures-feedback}
\end{figure}

\begin{figure}[h]
    \centering    \includegraphics[width=\linewidth]{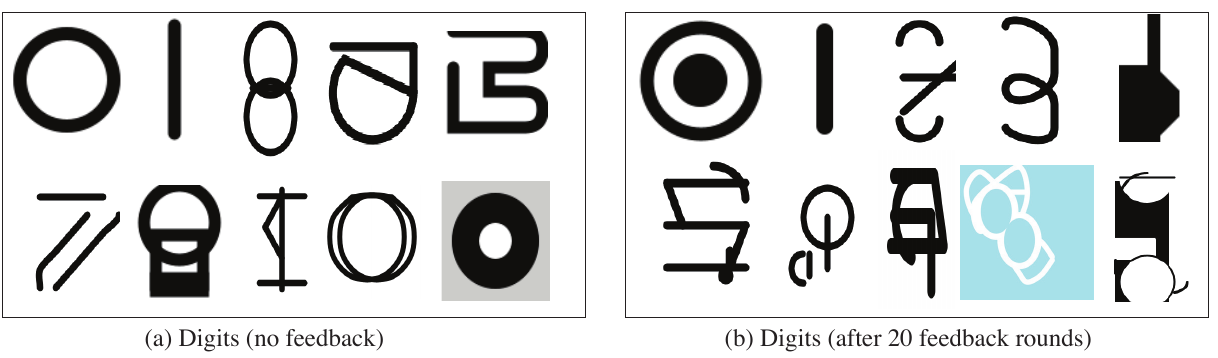}
    \caption{\textbf{Digits generation with feedback.} LLMs (GPT-3.5 in this case) fail to generate digits even with multiple feedback rounds. The images in both cases correspond to the digits 0-9.}
    \label{fig:failures-digits}
\end{figure}

\clearpage
\newpage
\subsection{Learning a vision system from text.}
We complement the experiments in Section 5 of the main paper with a comparison of each of the text models we test through the paper: Davinci, GPT-3.5 and GPT-4. In this case, we use 10k images for each of the datasets, and train and evaluate with a resolution of $192 \times 192$. We use a smaller network, ResNet-18, a smaller batch size of 8, and train for 500 epochs without MixUP. which allows us to test how good the raw original image content is.

In Tab.~\ref{tab:results_small_scale} we summarize the performance of the models when evaluated for classification on Imagenet-100, using the linear evaluation protocol. As can be seen, under this setting, the text models perform considerably worse than alternatives, which we attribute to the lack of texture, which the MixUP technique can overcome. Despite this, we can see that GPT-4 generated images outperform those from less capable models like Davinci and GPT-3.5, which perform similarly.

\begin{table}[htbp]
\centering
\begin{tabular}{|l|c|}
\hline
\textbf{Model} & \textbf{Top-1 I-100 accuracy (\%)} \\
\hline

Dead Leaves & 40.02 \\
StyleGAN & 43.94 \\
Fractals & 44.66 \\
Shaders & 46.22 \\
\hline
GPT-3.5 Turbo & 29.70 \\
Davinci & 30.14 \\
GPT-4 & 33.90 \\
\hline
\hline
Places365 & 48.66 \\
\hline

\end{tabular}
\caption{Top-1 Imagenet-100 accuracy for models trained using each of the synthetic datasets (including LLM's) and real images (Places).}
\label{tab:results_small_scale}
\end{table}

\begin{figure}[h]
     \centering
     \includegraphics[width=0.5\textwidth]{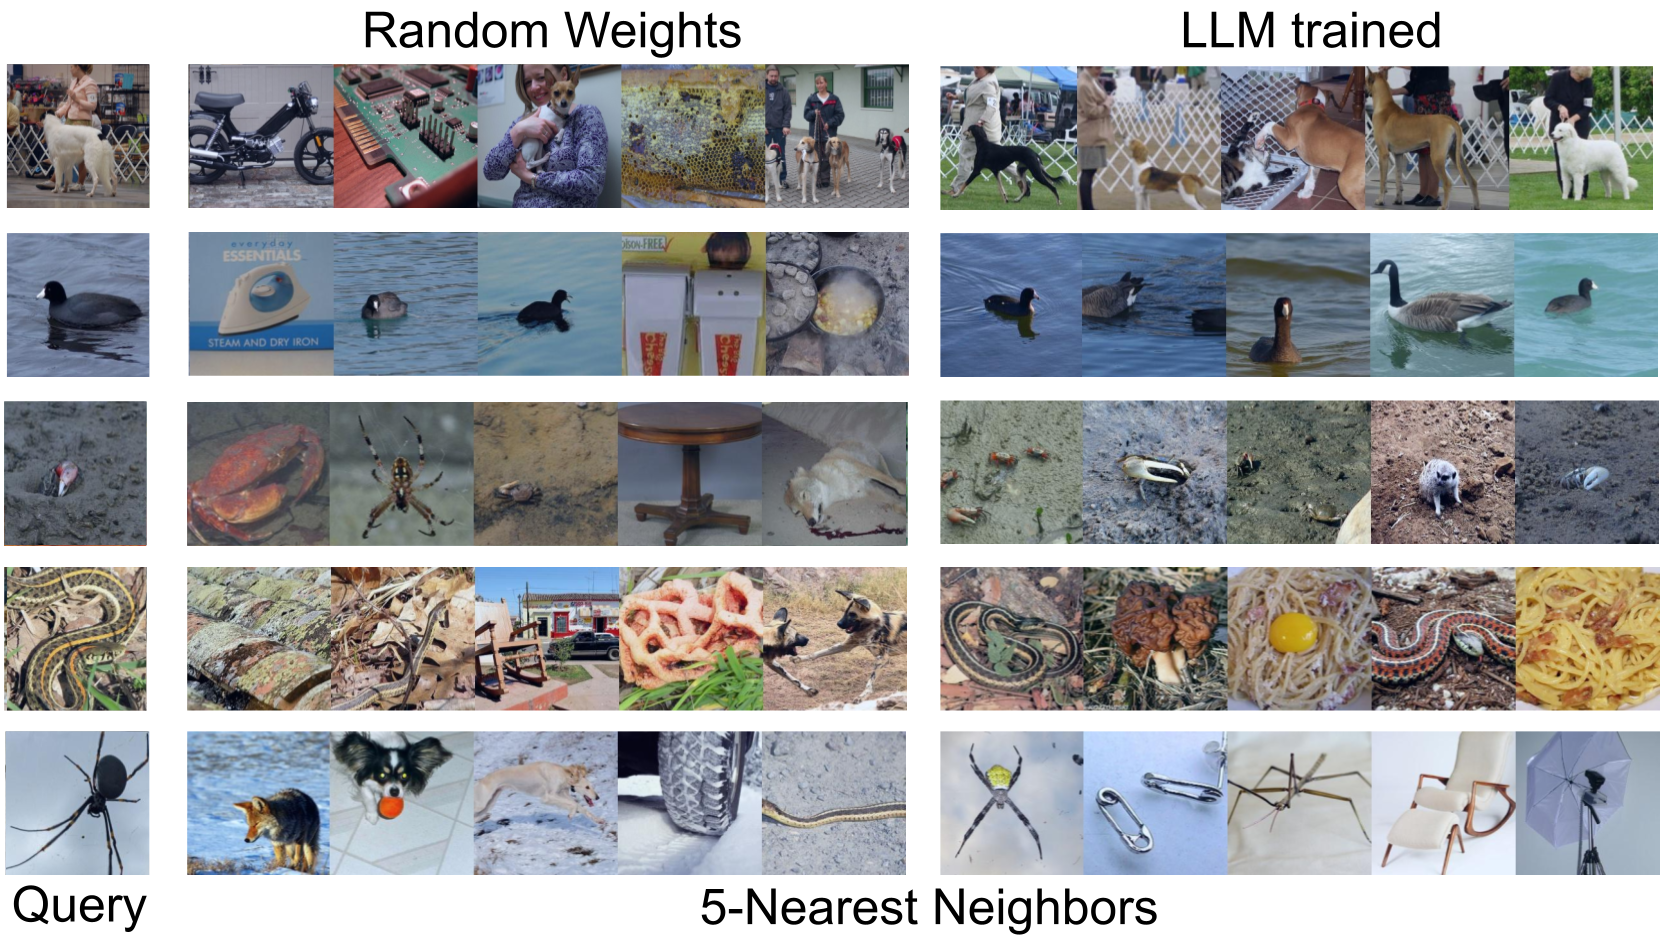}
     \caption{\textbf{Nearest Neighbors Retrieval on Imagenet-100.} Nearest neighbors on Imagenet-100 for a randomly initialized network and a network trained with our LLM-generated images without GPT-4 data.}
     \label{fig:nearest_neibhgors_LLM}
\end{figure}

\clearpage
\newpage
\subsection{Open-source models}

Open-source models –– Llama2 (chat 70B), GPTJ, and GPT2 fail at generating quality image-rendering code.

\paragraph{LLama2 (chat 70B).}

Llama2 successfully generated compilable code a significant percentage of the time, though the rate was very low with concepts of higher complexity in languages other than matplotlib. However, even when the code successfully produced an image the semantic accuracy of the generations was incredibly poor, matching part of the prompt at best on a very small fraction of cases and generating complete nonsense in all the others. We include some of the generated examples and the corresponding prompts in \cref{fig:generations-llama270b-shapes-matplotlib,fig:generations-llama270b-objects-tikz,fig:generations-llama270b-scenes-processing}

\paragraph{GPTJ and GPT2.}
GPTJ and GPT2 were not able to produce compilable code at all and often did not even yield code, with the generated text displaying significant pathologies and misalignment with the prompt.

\begin{figure}[h]
    \centering    \includegraphics[width=\linewidth,trim={0 42cm 0 0},clip]{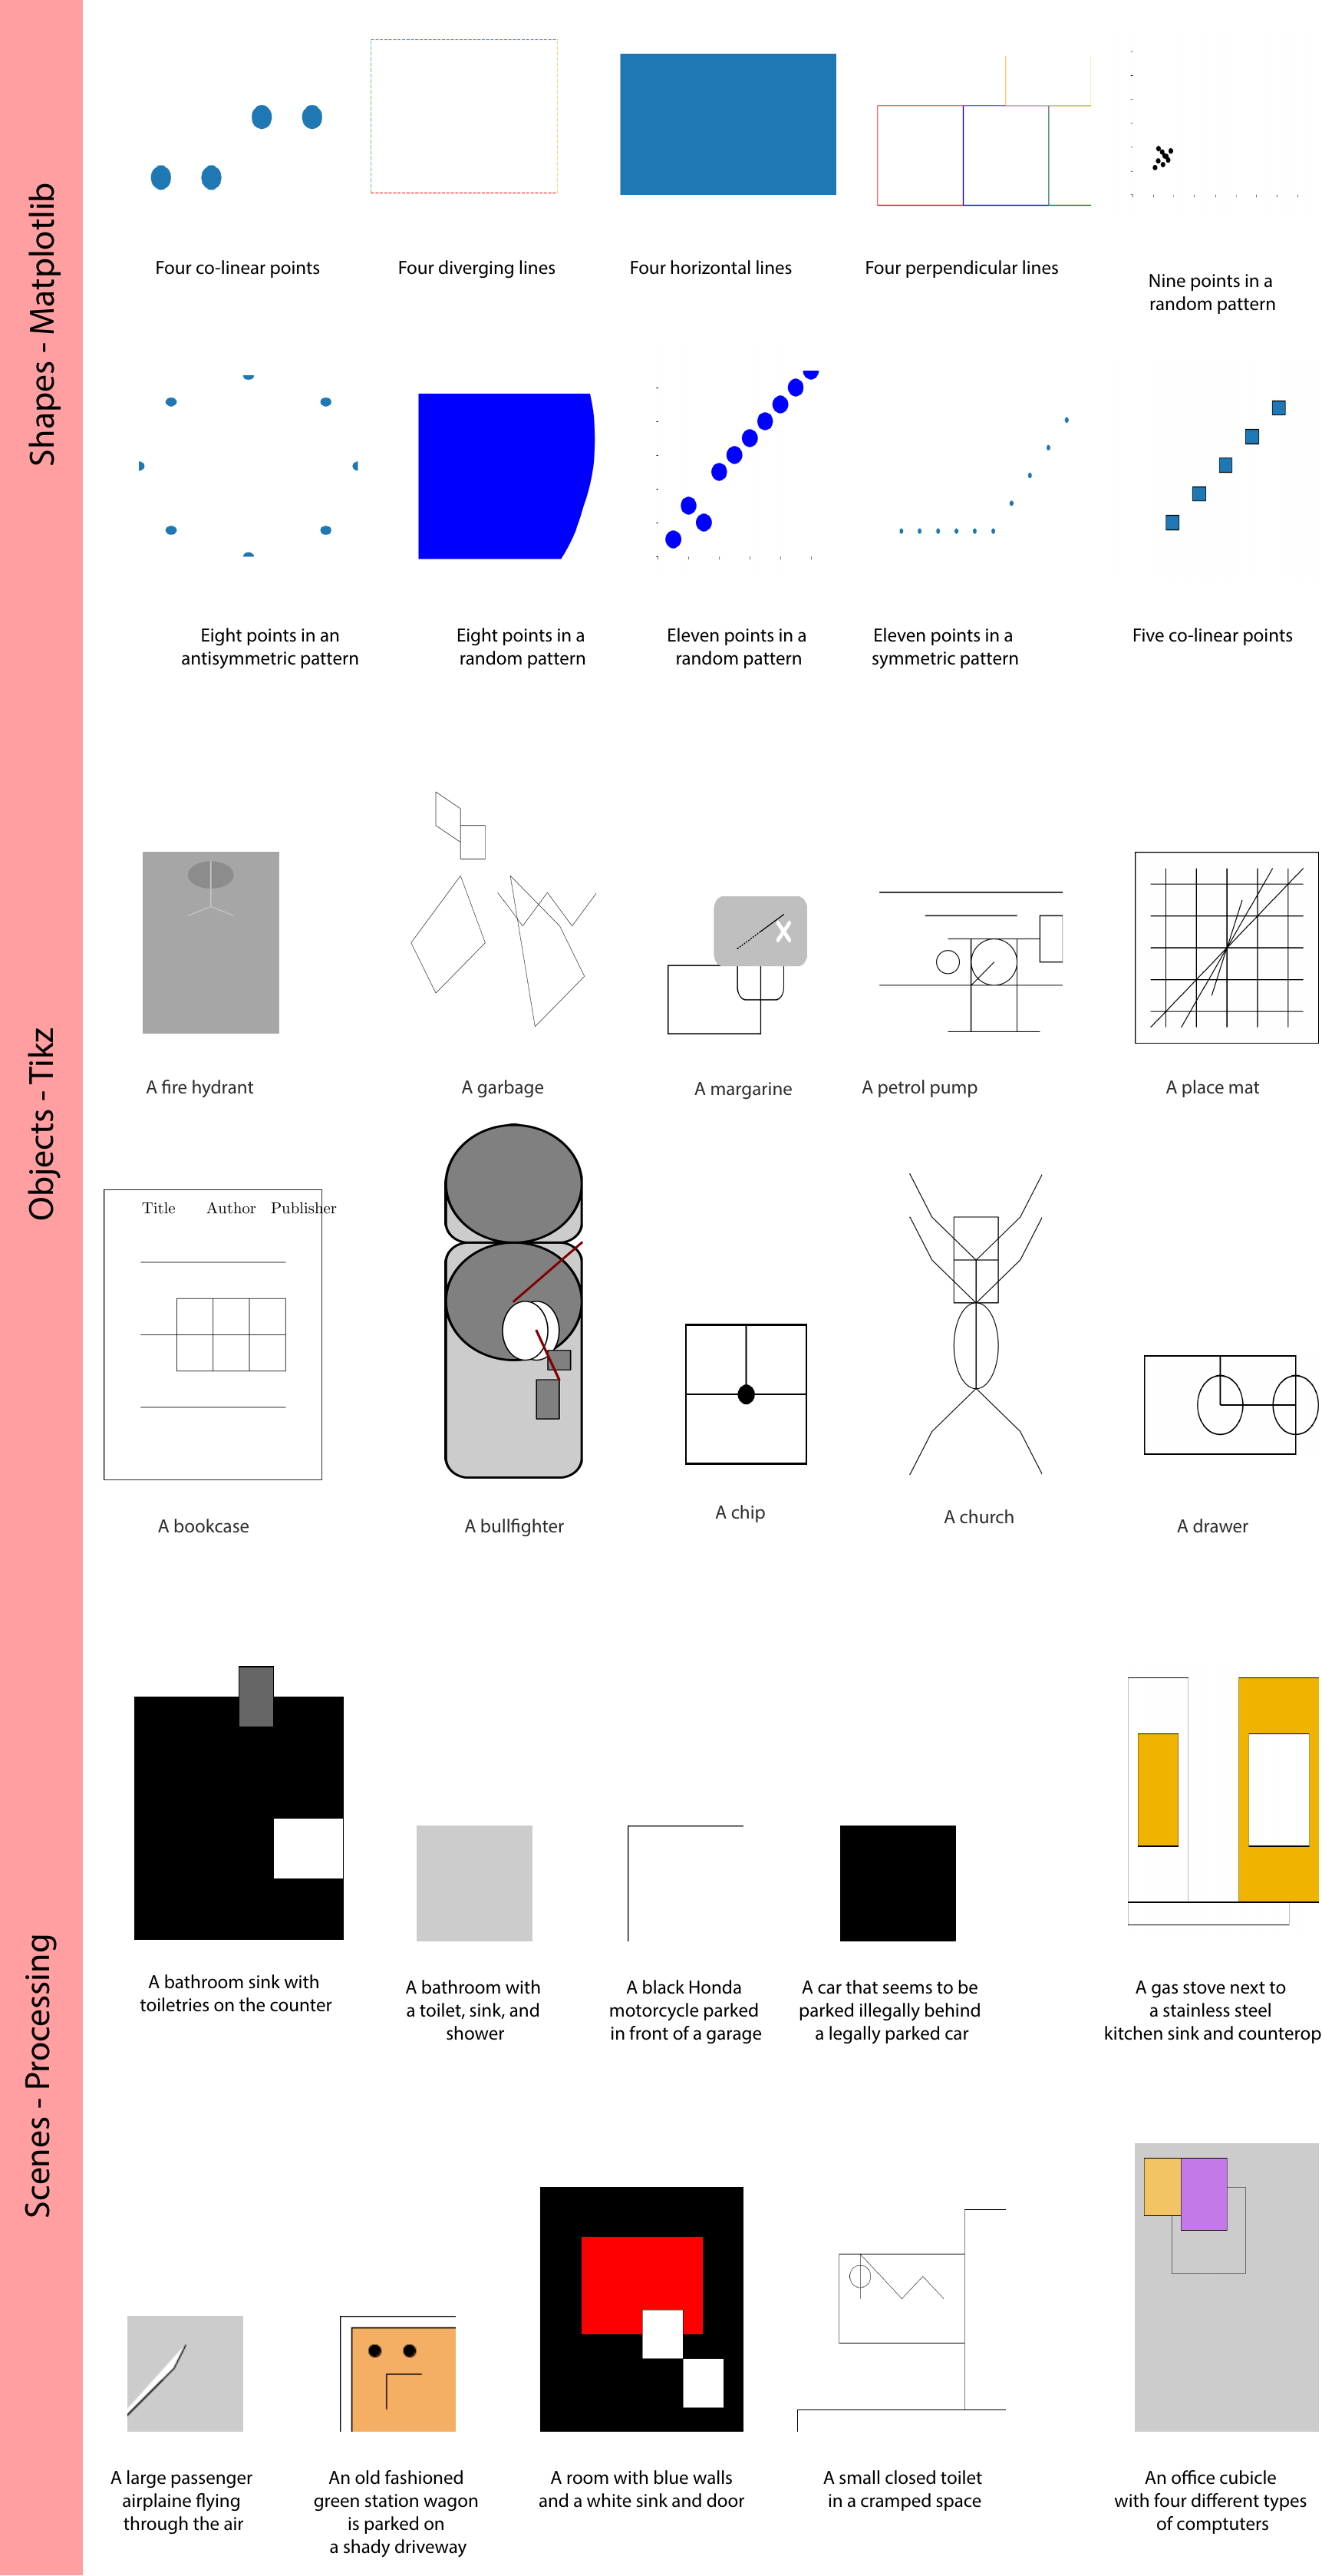}
    \caption{\textbf{Image generation with Llama-2-70B chat.} Shapes in Matplotlib.}
    \label{fig:generations-llama270b-shapes-matplotlib}
\end{figure}
\begin{figure}[h]
    \centering    \includegraphics[width=\linewidth,trim={0 22cm 0 17cm},clip]{figures/Llama2-examples-thin.pdf}
    \caption{\textbf{Image generation with Llama-2-70B chat.} Objects in Tikz.}
    \label{fig:generations-llama270b-objects-tikz}
\end{figure}
\begin{figure}[h]
    \centering    \includegraphics[width=\linewidth,trim={0 0 0 36cm},clip]{figures/Llama2-examples-thin.pdf}
    \caption{\textbf{Image generation with Llama-2-70B chat.} Scenes in Processing.}
    \label{fig:generations-llama270b-scenes-processing}
\end{figure}

\begin{lstlisting}[frame=single,style=base]
@User input:@ You are a helpful assistance and an excellent programmer. You output a script in the programming language "Processing" that draws what the user asks to draw. Remove any text. Use settings() instead of setup().Draw an image of a church.
\end{lstlisting}

\begin{lstlisting}[frame=single,style=base]
*GPTJ (run 1):* You are a helpful assistant and a very fine programmer. You output a script in the programming language "Processing" that draws what the user asks to draw. Remove any text. Use settings() instead of setup(). Draw an image of a church.

You are a smart and knowledgeable assistant. You output a script in the programming language "Processing" that draws what the user asks to draw. Remove any text. Use settings() instead of setup().Draw an image of a church.

You are a smart assistant and a fine programmer. You output a script in the programming language "Processing" that draws what the user asks to draw. Remove any text. Use settings() instead of setup().Draw an image of a church.

You are a smart assistant and a very fine programmer. You output a script in the programming language "Processing" that draws what the user asks to draw. Remove any text. Use settings() instead of setup().Draw an image of a church.

You are a knowledgeable assistant and a fine programmer. You output a script in the programming language "Processing" that draws what the user asks to draw. Remove any text. Use settings() instead of setup().Draw an image of a church.

You are a smart and helpful assistant. You output a script in the programming language "Processing" that draws what the user asks to draw. Remove any text. Use settings() instead of setup().Draw an image of a church.

A great assistant and a superb programmer. You output a script in the programming language "Processing" that draws what the user asks to draw. Remove any text. Use settings() instead of setup().Draw an image of a church.

You are a great assistant and a fine programmer. You output a script in the programming language "Processing" that draws what the user asks to draw. Remove any text. Use settings() instead of setup().Draw an image of a church.

You are a helpful assistant and a fine programmer. You output a script in the programming language "Processing" that draws what the user asks to draw. Remove any text. Use settings() instead of setup().Draw an image of a church.

You are a smart and knowledgeable assistant. You output a script in the programming language "Processing" that draws what the user asks to draw. Remove any text. Use settings() instead of setup(). Draw an image of a church.

...
\end{lstlisting}

\begin{lstlisting}[frame=single,style=base]
*GPTJ (run 2):*  You start off with a circle. You should create a class to define a circle. If you dont want the user to draw or see circles, you should use the class Circle. You should provide a constructor and a draw(), which should be called from the draw function.

When you finish the circle, you should draw a rectangle (which should be done in your draw function).

1. How do you draw circles?
2. What should the class look like?
3. How to you draw a rectangle?
4. How do you draw a circle and a rectangle?
5. How to you create two circles in different colors?
6. Give the output and explain/explain your answers in this exercise.You are a helpful assistance and an excellent programmer. You output a script in the programming language "Processing" that draws what the user asks to draw. Remove any text. Use settings() instead of setup().Draw an image of a church. Use fill() and stroke() instead of fillRect() and strokeRect().

...
\end{lstlisting}

\begin{lstlisting}[frame=single,style=base]
~GPT2 (run 1):~ You are a helpful assistance and an excellent programmer. You output a script in the programming language "Processing" that draws what the user asks to draw. Remove any text. Use settings() instead of setup().Draw an image of a church. Then use set<Cx> to change the color of the background with any text, or use the "rectangle to draw circle" to change your image with any circle. This will also let your users customize when you create the image instead of drawing with background decoration. I hope you love it.

You can use the following methods to draw blocks such as rectangles and rectangles above a text element. The example above will draw both an infinite circle and a circle.

using UnityEngine; using System.Collections.Generic; public class Program { public override void Run() { try { drawBlock(100, 125, "circle"); }catch(Exception e){ } } public void Toggle() { setCursor(2); } }

If you're using another game's engine as your server, you can also draw blocks here, using the same code from an Arduino, using the following example:
\end{lstlisting}

\begin{lstlisting}[frame=single,style=base]
~GPT2 (run 2):~ You are a helpful assistance and an excellent programmer. You output a script in the programming language "Processing" that draws what the user asks to draw. Remove any text. Use settings() instead of setup().Draw an image of a church.

The problem with drawing text is to draw a blank screen to allow the user from the screen. The user can draw the line of text while waiting some time to come at the cursor, if they want to.

The problem with drawing text is that this allows the user to see a black line. This is important since black lines can often appear in images. The user knows very fast enough so he might notice that the lines must be drawn to make the text white to work in the correct way.

The main problem with drawing characters like numbers is that the black lines can appear to be completely white and only draw the letters. However this can sometimes happen where there are other reasons for doing so, so the user might try to look over the color of the background.

I always keep an eye on these lines because sometimes text can become black at any time. The only time I ever see this happening is when the user scrolls to the right to get the scroll button.

Drawing the line of red

Use an image like this:

<div id="background" class="background color"> <table class="row col-md"> <tr><td align="left"> <h3>The script was made to show the black line</h3><p>This is called black lines. This can be one of the worst scripts ever written.</p><p>This script is created into the system for you.</p><img title="black line" src="//lollipopjs.githubusercontent.com/el/logo.png" alt="Red light"></p><div> <table class="table col-md" table-name="Table of contents" col-first="5" class="padding"> <tr><td align="left"><img src="//lollipopjs.githubusercontent.com/el/logo.png" alt="Red light"></img> </tr> </table> </div> A similar approach could be to draw a line of blue which just shows an actual line. This is called black-line lines.

After you have created the output file, you should see the error: Error: In any program you have this problem you must start with this warning message.

In a long time, when you have worked with the text in a file then the following is sometimes not an issue.

Error Code: Unable to start the file: Invalid input type. Input does not exist. Output type: XML output file failed to open to error. Input type: DAT input file failed to open to error. OutputType mismatch found: No input element from the '.input' module was specified for the input element ('input').

If you have made note of the trouble before writing the code, you can try writing down the problem and write it down the same way you wrote the error.
\end{lstlisting}
